# Supplementary material for: Garbage Collection for Rust: The Finalizer Frontier
Source: arXiv:2504.01841 source file (2025-09-30)
Supplement: Supplementary file 1 [file appendix_elision_mem_hsize_avg_1.tex]

\begin{tabular}{ll@{\hspace{6pt}}r@{\hspace{3pt}}l@{\hspace{6pt}}r@{\hspace{3pt}}l}
\toprule
Suite & Benchmark & \multicolumn{4}{c}{Avg. heap size} \\
 &  & \multicolumn{2}{c}{After} & \multicolumn{2}{c}{Before} \\
\midrule
\multirow{10}{*}{\rotatebox{90}{alacritty}} & Unicode & \scriptsize\textcolor{gray!60}{$\pm$69.838} & 4013.841 & \scriptsize\textcolor{gray!60}{$\pm$97.108} & 3925.449 \\
 & Scroll & \scriptsize\textcolor{gray!60}{$\pm$83.065} & 3947.345 & \scriptsize\textcolor{gray!60}{$\pm$108.988} & 3883.548 \\
 & Scroll Btm & \scriptsize\textcolor{gray!60}{$\pm$69.952} & 3944.248 & \scriptsize\textcolor{gray!60}{$\pm$61.957} & 3926.583 \\
 & Scroll Btm (small) & \scriptsize\textcolor{gray!60}{$\pm$65.867} & 3924.307 & \scriptsize\textcolor{gray!60}{$\pm$60.086} & 3931.525 \\
 & Light Cells & \scriptsize\textcolor{gray!60}{$\pm$92.187} & 3868.807 & \scriptsize\textcolor{gray!60}{$\pm$82.206} & 3938.587 \\
 & Scroll (fullscreen) & \scriptsize\textcolor{gray!60}{$\pm$316.790} & 6646.230 & \scriptsize\textcolor{gray!60}{$\pm$392.413} & 6639.241 \\
 & Scroll Top & \scriptsize\textcolor{gray!60}{$\pm$102.455} & 3995.875 & \scriptsize\textcolor{gray!60}{$\pm$106.698} & 4003.190 \\
 & Scroll Top (small) & \scriptsize\textcolor{gray!60}{$\pm$100.806} & 3931.125 & \scriptsize\textcolor{gray!60}{$\pm$65.535} & 3907.082 \\
 & Cur. Motion & \scriptsize\textcolor{gray!60}{$\pm$64.778} & 3909.177 & \scriptsize\textcolor{gray!60}{$\pm$220.881} & 3875.911 \\
 & Dense Cells & \scriptsize\textcolor{gray!60}{$\pm$86.474} & 3981.284 & \scriptsize\textcolor{gray!60}{$\pm$61.589} & 3930.283 \\
\midrule
\multirow{26}{*}{\rotatebox{90}{som-rs-ast}} & Loop & \scriptsize\textcolor{gray!60}{$\pm$8269.648} & 346515.951 & \scriptsize\textcolor{gray!60}{$\pm$17261.945} & 349002.871 \\
 & Mandelbrot & \scriptsize\textcolor{gray!60}{$\pm$2717.877} & 246937.506 & \scriptsize\textcolor{gray!60}{$\pm$3162.124} & 287322.410 \\
 & NBody & \scriptsize\textcolor{gray!60}{$\pm$2911.983} & 143679.243 & \scriptsize\textcolor{gray!60}{$\pm$2390.435} & 158384.360 \\
 & PageRank & \scriptsize\textcolor{gray!60}{$\pm$981.561} & 176080.104 & \scriptsize\textcolor{gray!60}{$\pm$1573.368} & 203624.492 \\
 & Permute & \scriptsize\textcolor{gray!60}{$\pm$8810.702} & 394868.592 & \scriptsize\textcolor{gray!60}{$\pm$44410.391} & 319817.974 \\
 & Queens & \scriptsize\textcolor{gray!60}{$\pm$11751.774} & 305997.606 & \scriptsize\textcolor{gray!60}{$\pm$15488.749} & 289840.231 \\
 & QuickSort & \scriptsize\textcolor{gray!60}{$\pm$14412.069} & 457245.723 & \scriptsize\textcolor{gray!60}{$\pm$17235.853} & 524142.686 \\
 & Recurse & \scriptsize\textcolor{gray!60}{$\pm$3768.892} & 431237.534 & \scriptsize\textcolor{gray!60}{$\pm$27632.072} & 440976.511 \\
 & Richards & \scriptsize\textcolor{gray!60}{$\pm$40997.123} & 1542715.020 & \scriptsize\textcolor{gray!60}{$\pm$115358.040} & 1293602.717 \\
 & List & \scriptsize\textcolor{gray!60}{$\pm$4760.732} & 162157.519 & \scriptsize\textcolor{gray!60}{$\pm$4183.955} & 251693.590 \\
 & JsonSmall & \scriptsize\textcolor{gray!60}{$\pm$1249.455} & 331208.395 & \scriptsize\textcolor{gray!60}{$\pm$34421.256} & 266788.914 \\
 & Bounce & \scriptsize\textcolor{gray!60}{$\pm$7225.595} & 385884.783 & \scriptsize\textcolor{gray!60}{$\pm$37763.804} & 299459.291 \\
 & BubbleSort & \scriptsize\textcolor{gray!60}{$\pm$4022.409} & 220185.596 & \scriptsize\textcolor{gray!60}{$\pm$6452.732} & 355947.310 \\
 & DeltaBlue & \scriptsize\textcolor{gray!60}{$\pm$5281.543} & 332058.469 & \scriptsize\textcolor{gray!60}{$\pm$31633.218} & 317319.460 \\
 & Dispatch & \scriptsize\textcolor{gray!60}{$\pm$7670.369} & 352244.761 & \scriptsize\textcolor{gray!60}{$\pm$21048.186} & 361585.674 \\
 & Fannkuch & \scriptsize\textcolor{gray!60}{$\pm$9823.564} & 377835.986 & \scriptsize\textcolor{gray!60}{$\pm$6138.023} & 435866.573 \\
 & Sieve & \scriptsize\textcolor{gray!60}{$\pm$5141.769} & 373029.129 & \scriptsize\textcolor{gray!60}{$\pm$22047.534} & 368917.173 \\
 & Fibonacci & \scriptsize\textcolor{gray!60}{$\pm$5479.066} & 613871.324 & \scriptsize\textcolor{gray!60}{$\pm$33503.200} & 405431.151 \\
 & FieldLoop & \scriptsize\textcolor{gray!60}{$\pm$6434.248} & 315572.299 & \scriptsize\textcolor{gray!60}{$\pm$14972.385} & 329331.274 \\
 & GraphSearch & \scriptsize\textcolor{gray!60}{$\pm$204.625} & 63953.863 & \scriptsize\textcolor{gray!60}{$\pm$4204.212} & 106218.045 \\
 & IntegerLoop & \scriptsize\textcolor{gray!60}{$\pm$444.583} & 335948.388 & \scriptsize\textcolor{gray!60}{$\pm$19150.082} & 327838.765 \\
 & Storage & \scriptsize\textcolor{gray!60}{$\pm$5479.314} & 199344.443 & \scriptsize\textcolor{gray!60}{$\pm$9773.034} & 210924.673 \\
 & Sum & \scriptsize\textcolor{gray!60}{$\pm$3195.460} & 313994.074 & \scriptsize\textcolor{gray!60}{$\pm$12039.544} & 342154.389 \\
 & Towers & \scriptsize\textcolor{gray!60}{$\pm$410.339} & 184286.193 & \scriptsize\textcolor{gray!60}{$\pm$2004.490} & 185603.225 \\
 & TreeSort & \scriptsize\textcolor{gray!60}{$\pm$1359.826} & 103198.617 & \scriptsize\textcolor{gray!60}{$\pm$5604.504} & 96007.790 \\
 & WhileLoop & \scriptsize\textcolor{gray!60}{$\pm$2759.670} & 268439.769 & \scriptsize\textcolor{gray!60}{$\pm$14779.540} & 282485.147 \\
\midrule
\multirow{7}{*}{\rotatebox{90}{fd}} & No Pattern & \scriptsize\textcolor{gray!60}{$\pm$688.526} & 53764.817 & \scriptsize\textcolor{gray!60}{$\pm$1685.296} & 52634.618 \\
 & Simple & \scriptsize\textcolor{gray!60}{$\pm$127.897} & 23168.290 & \scriptsize\textcolor{gray!60}{$\pm$635.343} & 22226.950 \\
 & Simple (-HI) & \scriptsize\textcolor{gray!60}{$\pm$1003.795} & 10086.630 & \scriptsize\textcolor{gray!60}{$\pm$1458.040} & 13322.517 \\
 & File Type & \scriptsize\textcolor{gray!60}{$\pm$1222.583} & 11259.742 & \scriptsize\textcolor{gray!60}{$\pm$317.459} & 13607.795 \\
 & Cmd Exec. & \scriptsize\textcolor{gray!60}{$\pm$504.288} & 18239.394 & \scriptsize\textcolor{gray!60}{$\pm$529.626} & 18847.434 \\
 & Cmd Exec. (large) & \scriptsize\textcolor{gray!60}{$\pm$725.117} & 18573.598 & \scriptsize\textcolor{gray!60}{$\pm$967.961} & 20665.791 \\
 & File Extension & \scriptsize\textcolor{gray!60}{$\pm$813.347} & 12160.342 & \scriptsize\textcolor{gray!60}{$\pm$519.194} & 12214.696 \\
\bottomrule
\end{tabular}
