# Supplementary material for: Garbage Collection for Rust: The Finalizer Frontier
Source: arXiv:2504.01841 source file (2025-09-30)
Supplement: Supplementary file 2 [file appendix_elision_mem_hsize_avg_2.tex]

\begin{tabular}{ll@{\hspace{6pt}}r@{\hspace{3pt}}l@{\hspace{6pt}}r@{\hspace{3pt}}l}
\toprule
Suite & Benchmark & \multicolumn{4}{c}{Avg. heap size} \\
 &  & \multicolumn{2}{c}{After} & \multicolumn{2}{c}{Before} \\
\midrule
\multirow{4}{*}{\rotatebox{90}{grmtools}} & Spring & \scriptsize\textcolor{gray!60}{$\pm$23907.967} & 1097942.375 & \scriptsize\textcolor{gray!60}{$\pm$2302.476} & 1839017.329 \\
 & Eclipse & \scriptsize\textcolor{gray!60}{$\pm$32582.551} & 1108090.312 & \scriptsize\textcolor{gray!60}{$\pm$9742.834} & 2090203.507 \\
 & Hadoop & \scriptsize\textcolor{gray!60}{$\pm$38725.045} & 817330.455 & \scriptsize\textcolor{gray!60}{$\pm$1955.807} & 1972942.886 \\
 & Jenkins & \scriptsize\textcolor{gray!60}{$\pm$29061.374} & 1016114.022 & \scriptsize\textcolor{gray!60}{$\pm$4941.839} & 1977358.953 \\
\midrule
\multirow{26}{*}{\rotatebox{90}{som-rs-bc}} & Loop & \scriptsize\textcolor{gray!60}{$\pm$7.493} & 126762.910 & \scriptsize\textcolor{gray!60}{$\pm$6948.434} & 152972.156 \\
 & Mandelbrot & \scriptsize\textcolor{gray!60}{$\pm$24.492} & 84402.450 & \scriptsize\textcolor{gray!60}{$\pm$4614.270} & 94760.553 \\
 & NBody & \scriptsize\textcolor{gray!60}{$\pm$33.018} & 50481.813 & \scriptsize\textcolor{gray!60}{$\pm$1950.787} & 63265.382 \\
 & PageRank & \scriptsize\textcolor{gray!60}{$\pm$648.746} & 54537.441 & \scriptsize\textcolor{gray!60}{$\pm$71.687} & 72634.939 \\
 & Permute & \scriptsize\textcolor{gray!60}{$\pm$31.497} & 115065.566 & \scriptsize\textcolor{gray!60}{$\pm$5822.686} & 130822.161 \\
 & Queens & \scriptsize\textcolor{gray!60}{$\pm$31.112} & 140824.532 & \scriptsize\textcolor{gray!60}{$\pm$5515.639} & 161433.159 \\
 & QuickSort & \scriptsize\textcolor{gray!60}{$\pm$129.564} & 183951.869 & \scriptsize\textcolor{gray!60}{$\pm$6466.309} & 190749.021 \\
 & Recurse & \scriptsize\textcolor{gray!60}{$\pm$0.697} & 153519.859 & \scriptsize\textcolor{gray!60}{$\pm$8768.938} & 176841.293 \\
 & Richards & \scriptsize\textcolor{gray!60}{$\pm$33.257} & 511643.759 & \scriptsize\textcolor{gray!60}{$\pm$32613.893} & 619204.556 \\
 & List & \scriptsize\textcolor{gray!60}{$\pm$36.676} & 103760.499 & \scriptsize\textcolor{gray!60}{$\pm$6983.268} & 112793.829 \\
 & JsonSmall & \scriptsize\textcolor{gray!60}{$\pm$6443.944} & 144934.994 & \scriptsize\textcolor{gray!60}{$\pm$6560.952} & 173234.539 \\
 & Bounce & \scriptsize\textcolor{gray!60}{$\pm$288.124} & 140613.639 & \scriptsize\textcolor{gray!60}{$\pm$5331.593} & 144643.208 \\
 & BubbleSort & \scriptsize\textcolor{gray!60}{$\pm$30.037} & 120845.625 & \scriptsize\textcolor{gray!60}{$\pm$5671.862} & 130716.887 \\
 & DeltaBlue & \scriptsize\textcolor{gray!60}{$\pm$2112.400} & 141661.252 & \scriptsize\textcolor{gray!60}{$\pm$835.316} & 196051.330 \\
 & Dispatch & \scriptsize\textcolor{gray!60}{$\pm$7.856} & 143742.898 & \scriptsize\textcolor{gray!60}{$\pm$7691.397} & 173079.905 \\
 & Fannkuch & \scriptsize\textcolor{gray!60}{$\pm$26.966} & 121627.373 & \scriptsize\textcolor{gray!60}{$\pm$5647.061} & 148030.241 \\
 & Sieve & \scriptsize\textcolor{gray!60}{$\pm$4112.561} & 117440.060 & \scriptsize\textcolor{gray!60}{$\pm$5571.861} & 140518.774 \\
 & Fibonacci & \scriptsize\textcolor{gray!60}{$\pm$26.923} & 184433.201 & \scriptsize\textcolor{gray!60}{$\pm$9852.697} & 215582.643 \\
 & FieldLoop & \scriptsize\textcolor{gray!60}{$\pm$7.622} & 93399.082 & \scriptsize\textcolor{gray!60}{$\pm$4992.331} & 109466.987 \\
 & GraphSearch & \scriptsize\textcolor{gray!60}{$\pm$772.458} & 25507.239 & \scriptsize\textcolor{gray!60}{$\pm$1496.735} & 47287.859 \\
 & IntegerLoop & \scriptsize\textcolor{gray!60}{$\pm$17.970} & 122952.775 & \scriptsize\textcolor{gray!60}{$\pm$6266.672} & 145322.005 \\
 & Storage & \scriptsize\textcolor{gray!60}{$\pm$3056.220} & 90556.627 & \scriptsize\textcolor{gray!60}{$\pm$1852.165} & 75275.884 \\
 & Sum & \scriptsize\textcolor{gray!60}{$\pm$7.018} & 123263.907 & \scriptsize\textcolor{gray!60}{$\pm$5772.449} & 142852.585 \\
 & Towers & \scriptsize\textcolor{gray!60}{$\pm$22.518} & 61724.734 & \scriptsize\textcolor{gray!60}{$\pm$3582.042} & 71366.053 \\
 & TreeSort & \scriptsize\textcolor{gray!60}{$\pm$1005.977} & 46873.581 & \scriptsize\textcolor{gray!60}{$\pm$2448.005} & 59305.510 \\
 & WhileLoop & \scriptsize\textcolor{gray!60}{$\pm$6.099} & 100968.590 & \scriptsize\textcolor{gray!60}{$\pm$3765.500} & 137993.571 \\
\midrule
\multirow{13}{*}{\rotatebox{90}{ripgrep}} & Literal (mmap, -i) & \scriptsize\textcolor{gray!60}{$\pm$599.164} & 18116.605 & \scriptsize\textcolor{gray!60}{$\pm$1675.689} & 30116.644 \\
 & Literal (default) & \scriptsize\textcolor{gray!60}{$\pm$427.961} & 15624.509 & \scriptsize\textcolor{gray!60}{$\pm$1731.812} & 27440.318 \\
 & Literal (mmap) & \scriptsize\textcolor{gray!60}{$\pm$292.023} & 16602.010 & \scriptsize\textcolor{gray!60}{$\pm$1872.392} & 27574.413 \\
 & Literal (regex) & \scriptsize\textcolor{gray!60}{$\pm$508.393} & 15848.717 & \scriptsize\textcolor{gray!60}{$\pm$1952.530} & 27102.240 \\
 & Literal (-i) & \scriptsize\textcolor{gray!60}{$\pm$263.752} & 18901.368 & \scriptsize\textcolor{gray!60}{$\pm$1428.294} & 28549.987 \\
 & UTF Greek & \scriptsize\textcolor{gray!60}{$\pm$618.021} & 18072.062 & \scriptsize\textcolor{gray!60}{$\pm$1139.482} & 28051.731 \\
 & UTF Greek (-i) & \scriptsize\textcolor{gray!60}{$\pm$246.410} & 19543.629 & \scriptsize\textcolor{gray!60}{$\pm$1369.732} & 28147.406 \\
 & UTF Word & \scriptsize\textcolor{gray!60}{$\pm$149.430} & 19120.233 & \scriptsize\textcolor{gray!60}{$\pm$1584.169} & 29355.825 \\
 & UTF Word (alt.) & \scriptsize\textcolor{gray!60}{$\pm$528.154} & 16040.239 & \scriptsize\textcolor{gray!60}{$\pm$1512.979} & 25541.969 \\
 & Word & \scriptsize\textcolor{gray!60}{$\pm$441.139} & 16592.486 & \scriptsize\textcolor{gray!60}{$\pm$2039.723} & 29626.525 \\
 & Literal & \scriptsize\textcolor{gray!60}{$\pm$316.648} & 15924.715 & \scriptsize\textcolor{gray!60}{$\pm$1478.226} & 27007.278 \\
 & Alternates & \scriptsize\textcolor{gray!60}{$\pm$336.174} & 16683.091 & \scriptsize\textcolor{gray!60}{$\pm$1651.590} & 29775.150 \\
 & Alternates (-i) & \scriptsize\textcolor{gray!60}{$\pm$493.809} & 18528.434 & \scriptsize\textcolor{gray!60}{$\pm$1651.208} & 31496.261 \\
\bottomrule
\end{tabular}
