# Supplementary material for: Garbage Collection for Rust: The Finalizer Frontier
Source: arXiv:2504.01841 source file (2025-09-30)
Supplement: Supplementary file 3 [file appendix_elision_obj_allocd_gc_1.tex]

\begin{tabular}{ll@{\hspace{6pt}}r@{\hspace{3pt}}l@{\hspace{6pt}}r@{\hspace{3pt}}l}
\toprule
Suite & Benchmark & \multicolumn{4}{c}{None} \\
 &  & \multicolumn{2}{c}{After} & \multicolumn{2}{c}{Before} \\
\midrule
\multirow{10}{*}{\rotatebox{90}{alacritty}} & Unicode & \scriptsize\textcolor{gray!60}{$\pm$0.000} & 0.002 & \scriptsize\textcolor{gray!60}{$\pm$0.000} & 0.002 \\
 & Scroll & \scriptsize\textcolor{gray!60}{$\pm$0.000} & 0.002 & \scriptsize\textcolor{gray!60}{$\pm$0.000} & 0.002 \\
 & Scroll Btm & \scriptsize\textcolor{gray!60}{$\pm$0.000} & 0.002 & \scriptsize\textcolor{gray!60}{$\pm$0.000} & 0.002 \\
 & Scroll Btm (small) & \scriptsize\textcolor{gray!60}{$\pm$0.000} & 0.002 & \scriptsize\textcolor{gray!60}{$\pm$0.000} & 0.002 \\
 & Light Cells & \scriptsize\textcolor{gray!60}{$\pm$0.000} & 0.002 & \scriptsize\textcolor{gray!60}{$\pm$0.000} & 0.002 \\
 & Scroll (fullscreen) & \scriptsize\textcolor{gray!60}{$\pm$0.000} & 0.002 & \scriptsize\textcolor{gray!60}{$\pm$0.000} & 0.002 \\
 & Scroll Top & \scriptsize\textcolor{gray!60}{$\pm$0.000} & 0.002 & \scriptsize\textcolor{gray!60}{$\pm$0.000} & 0.002 \\
 & Scroll Top (small) & \scriptsize\textcolor{gray!60}{$\pm$0.000} & 0.002 & \scriptsize\textcolor{gray!60}{$\pm$0.000} & 0.002 \\
 & Cur. Motion & \scriptsize\textcolor{gray!60}{$\pm$0.000} & 0.002 & \scriptsize\textcolor{gray!60}{$\pm$0.000} & 0.002 \\
 & Dense Cells & \scriptsize\textcolor{gray!60}{$\pm$0.000} & 0.002 & \scriptsize\textcolor{gray!60}{$\pm$0.000} & 0.002 \\
\midrule
\multirow{26}{*}{\rotatebox{90}{som-rs-ast}} & Loop & \scriptsize\textcolor{gray!60}{$\pm$0.000} & 1653.042 & \scriptsize\textcolor{gray!60}{$\pm$0.000} & 1653.042 \\
 & Mandelbrot & \scriptsize\textcolor{gray!60}{$\pm$0.000} & 1203.646 & \scriptsize\textcolor{gray!60}{$\pm$0.000} & 1203.646 \\
 & NBody & \scriptsize\textcolor{gray!60}{$\pm$0.000} & 573.375 & \scriptsize\textcolor{gray!60}{$\pm$0.000} & 573.375 \\
 & PageRank & \scriptsize\textcolor{gray!60}{$\pm$0.000} & 743.852 & \scriptsize\textcolor{gray!60}{$\pm$0.000} & 743.852 \\
 & Permute & \scriptsize\textcolor{gray!60}{$\pm$0.000} & 1358.043 & \scriptsize\textcolor{gray!60}{$\pm$0.000} & 1358.043 \\
 & Queens & \scriptsize\textcolor{gray!60}{$\pm$0.000} & 1682.345 & \scriptsize\textcolor{gray!60}{$\pm$0.000} & 1682.345 \\
 & QuickSort & \scriptsize\textcolor{gray!60}{$\pm$0.000} & 2717.395 & \scriptsize\textcolor{gray!60}{$\pm$0.000} & 2717.395 \\
 & Recurse & \scriptsize\textcolor{gray!60}{$\pm$0.000} & 1884.932 & \scriptsize\textcolor{gray!60}{$\pm$0.000} & 1884.932 \\
 & Richards & \scriptsize\textcolor{gray!60}{$\pm$0.000} & 7290.035 & \scriptsize\textcolor{gray!60}{$\pm$0.000} & 7290.035 \\
 & List & \scriptsize\textcolor{gray!60}{$\pm$0.000} & 1427.299 & \scriptsize\textcolor{gray!60}{$\pm$0.000} & 1427.299 \\
 & JsonSmall & \scriptsize\textcolor{gray!60}{$\pm$0.000} & 2749.241 & \scriptsize\textcolor{gray!60}{$\pm$0.000} & 2749.241 \\
 & Bounce & \scriptsize\textcolor{gray!60}{$\pm$0.000} & 1739.229 & \scriptsize\textcolor{gray!60}{$\pm$0.000} & 1739.229 \\
 & BubbleSort & \scriptsize\textcolor{gray!60}{$\pm$0.000} & 1512.284 & \scriptsize\textcolor{gray!60}{$\pm$0.000} & 1512.284 \\
 & DeltaBlue & \scriptsize\textcolor{gray!60}{$\pm$0.000} & 2195.197 & \scriptsize\textcolor{gray!60}{$\pm$0.000} & 2195.197 \\
 & Dispatch & \scriptsize\textcolor{gray!60}{$\pm$0.000} & 1801.042 & \scriptsize\textcolor{gray!60}{$\pm$0.000} & 1801.042 \\
 & Fannkuch & \scriptsize\textcolor{gray!60}{$\pm$0.000} & 1615.422 & \scriptsize\textcolor{gray!60}{$\pm$0.000} & 1615.422 \\
 & Sieve & \scriptsize\textcolor{gray!60}{$\pm$0.000} & 1856.302 & \scriptsize\textcolor{gray!60}{$\pm$0.000} & 1856.302 \\
 & Fibonacci & \scriptsize\textcolor{gray!60}{$\pm$0.000} & 2585.992 & \scriptsize\textcolor{gray!60}{$\pm$0.000} & 2585.992 \\
 & FieldLoop & \scriptsize\textcolor{gray!60}{$\pm$0.000} & 1200.926 & \scriptsize\textcolor{gray!60}{$\pm$0.000} & 1200.926 \\
 & GraphSearch & \scriptsize\textcolor{gray!60}{$\pm$0.000} & 652.493 & \scriptsize\textcolor{gray!60}{$\pm$0.000} & 652.493 \\
 & IntegerLoop & \scriptsize\textcolor{gray!60}{$\pm$0.000} & 1600.966 & \scriptsize\textcolor{gray!60}{$\pm$0.000} & 1600.966 \\
 & Storage & \scriptsize\textcolor{gray!60}{$\pm$0.000} & 1461.648 & \scriptsize\textcolor{gray!60}{$\pm$0.000} & 1461.648 \\
 & Sum & \scriptsize\textcolor{gray!60}{$\pm$0.000} & 1601.522 & \scriptsize\textcolor{gray!60}{$\pm$0.000} & 1601.522 \\
 & Towers & \scriptsize\textcolor{gray!60}{$\pm$0.000} & 737.180 & \scriptsize\textcolor{gray!60}{$\pm$0.000} & 737.180 \\
 & TreeSort & \scriptsize\textcolor{gray!60}{$\pm$0.000} & 847.854 & \scriptsize\textcolor{gray!60}{$\pm$0.000} & 847.854 \\
 & WhileLoop & \scriptsize\textcolor{gray!60}{$\pm$0.000} & 1605.912 & \scriptsize\textcolor{gray!60}{$\pm$0.000} & 1605.912 \\
\midrule
\multirow{7}{*}{\rotatebox{90}{fd}} & No Pattern & \scriptsize\textcolor{gray!60}{$\pm$0.519} & 22.088 & \scriptsize\textcolor{gray!60}{$\pm$1.584} & 21.960 \\
 & Simple & \scriptsize\textcolor{gray!60}{$\pm$0.000} & 0.013 & \scriptsize\textcolor{gray!60}{$\pm$0.000} & 0.013 \\
 & Simple (-HI) & \scriptsize\textcolor{gray!60}{$\pm$0.000} & 0.013 & \scriptsize\textcolor{gray!60}{$\pm$0.000} & 0.013 \\
 & File Type & \scriptsize\textcolor{gray!60}{$\pm$0.001} & 0.034 & \scriptsize\textcolor{gray!60}{$\pm$0.001} & 0.034 \\
 & Cmd Exec. & \scriptsize\textcolor{gray!60}{$\pm$0.002} & 0.032 & \scriptsize\textcolor{gray!60}{$\pm$0.001} & 0.032 \\
 & Cmd Exec. (large) & \scriptsize\textcolor{gray!60}{$\pm$0.002} & 0.033 & \scriptsize\textcolor{gray!60}{$\pm$0.001} & 0.032 \\
 & File Extension & \scriptsize\textcolor{gray!60}{$\pm$0.000} & 0.022 & \scriptsize\textcolor{gray!60}{$\pm$0.000} & 0.022 \\
\bottomrule
\end{tabular}
