# Supplementary material for: Garbage Collection for Rust: The Finalizer Frontier
Source: arXiv:2504.01841 source file (2025-09-30)
Supplement: Supplementary file 4 [file appendix_elision_obj_allocd_gc_2.tex]

\begin{tabular}{ll@{\hspace{6pt}}r@{\hspace{3pt}}l@{\hspace{6pt}}r@{\hspace{3pt}}l}
\toprule
Suite & Benchmark & \multicolumn{4}{c}{None} \\
 &  & \multicolumn{2}{c}{After} & \multicolumn{2}{c}{Before} \\
\midrule
\multirow{4}{*}{\rotatebox{90}{grmtools}} & Spring & \scriptsize\textcolor{gray!60}{$\pm$11.201} & 2212.860 & \scriptsize\textcolor{gray!60}{$\pm$13.045} & 2214.817 \\
 & Eclipse & \scriptsize\textcolor{gray!60}{$\pm$346.179} & 9676.620 & \scriptsize\textcolor{gray!60}{$\pm$352.574} & 9670.023 \\
 & Hadoop & \scriptsize\textcolor{gray!60}{$\pm$6.502} & 2523.759 & \scriptsize\textcolor{gray!60}{$\pm$7.213} & 2522.361 \\
 & Jenkins & \scriptsize\textcolor{gray!60}{$\pm$43.066} & 6456.846 & \scriptsize\textcolor{gray!60}{$\pm$82.330} & 6404.411 \\
\midrule
\multirow{26}{*}{\rotatebox{90}{som-rs-bc}} & Loop & \scriptsize\textcolor{gray!60}{$\pm$0.000} & 1653.329 & \scriptsize\textcolor{gray!60}{$\pm$0.000} & 1653.329 \\
 & Mandelbrot & \scriptsize\textcolor{gray!60}{$\pm$0.000} & 1203.951 & \scriptsize\textcolor{gray!60}{$\pm$0.000} & 1203.951 \\
 & NBody & \scriptsize\textcolor{gray!60}{$\pm$0.000} & 573.679 & \scriptsize\textcolor{gray!60}{$\pm$0.000} & 573.679 \\
 & PageRank & \scriptsize\textcolor{gray!60}{$\pm$0.000} & 744.209 & \scriptsize\textcolor{gray!60}{$\pm$0.000} & 744.209 \\
 & Permute & \scriptsize\textcolor{gray!60}{$\pm$0.000} & 1358.326 & \scriptsize\textcolor{gray!60}{$\pm$0.000} & 1358.326 \\
 & Queens & \scriptsize\textcolor{gray!60}{$\pm$0.000} & 1682.634 & \scriptsize\textcolor{gray!60}{$\pm$0.000} & 1682.634 \\
 & QuickSort & \scriptsize\textcolor{gray!60}{$\pm$0.000} & 2717.719 & \scriptsize\textcolor{gray!60}{$\pm$0.000} & 2717.719 \\
 & Recurse & \scriptsize\textcolor{gray!60}{$\pm$0.000} & 1885.213 & \scriptsize\textcolor{gray!60}{$\pm$0.000} & 1885.213 \\
 & Richards & \scriptsize\textcolor{gray!60}{$\pm$0.000} & 7290.453 & \scriptsize\textcolor{gray!60}{$\pm$0.000} & 7290.453 \\
 & List & \scriptsize\textcolor{gray!60}{$\pm$0.000} & 1427.596 & \scriptsize\textcolor{gray!60}{$\pm$0.000} & 1427.596 \\
 & JsonSmall & \scriptsize\textcolor{gray!60}{$\pm$0.000} & 2579.765 & \scriptsize\textcolor{gray!60}{$\pm$0.000} & 2579.765 \\
 & Bounce & \scriptsize\textcolor{gray!60}{$\pm$0.000} & 1739.529 & \scriptsize\textcolor{gray!60}{$\pm$0.000} & 1739.529 \\
 & BubbleSort & \scriptsize\textcolor{gray!60}{$\pm$0.000} & 1512.596 & \scriptsize\textcolor{gray!60}{$\pm$0.000} & 1512.596 \\
 & DeltaBlue & \scriptsize\textcolor{gray!60}{$\pm$0.000} & 2195.841 & \scriptsize\textcolor{gray!60}{$\pm$0.000} & 2195.841 \\
 & Dispatch & \scriptsize\textcolor{gray!60}{$\pm$0.000} & 1801.323 & \scriptsize\textcolor{gray!60}{$\pm$0.000} & 1801.323 \\
 & Fannkuch & \scriptsize\textcolor{gray!60}{$\pm$0.000} & 1615.719 & \scriptsize\textcolor{gray!60}{$\pm$0.000} & 1615.719 \\
 & Sieve & \scriptsize\textcolor{gray!60}{$\pm$0.000} & 1856.589 & \scriptsize\textcolor{gray!60}{$\pm$0.000} & 1856.589 \\
 & Fibonacci & \scriptsize\textcolor{gray!60}{$\pm$0.000} & 2586.273 & \scriptsize\textcolor{gray!60}{$\pm$0.000} & 2586.273 \\
 & FieldLoop & \scriptsize\textcolor{gray!60}{$\pm$0.000} & 1201.209 & \scriptsize\textcolor{gray!60}{$\pm$0.000} & 1201.209 \\
 & GraphSearch & \scriptsize\textcolor{gray!60}{$\pm$0.000} & 652.817 & \scriptsize\textcolor{gray!60}{$\pm$0.000} & 652.817 \\
 & IntegerLoop & \scriptsize\textcolor{gray!60}{$\pm$0.000} & 1601.247 & \scriptsize\textcolor{gray!60}{$\pm$0.000} & 1601.247 \\
 & Storage & \scriptsize\textcolor{gray!60}{$\pm$0.000} & 1461.938 & \scriptsize\textcolor{gray!60}{$\pm$0.000} & 1461.938 \\
 & Sum & \scriptsize\textcolor{gray!60}{$\pm$0.000} & 1601.805 & \scriptsize\textcolor{gray!60}{$\pm$0.000} & 1601.805 \\
 & Towers & \scriptsize\textcolor{gray!60}{$\pm$0.000} & 737.473 & \scriptsize\textcolor{gray!60}{$\pm$0.000} & 737.473 \\
 & TreeSort & \scriptsize\textcolor{gray!60}{$\pm$0.000} & 848.185 & \scriptsize\textcolor{gray!60}{$\pm$0.000} & 848.185 \\
 & WhileLoop & \scriptsize\textcolor{gray!60}{$\pm$0.000} & 1606.199 & \scriptsize\textcolor{gray!60}{$\pm$0.000} & 1606.199 \\
\midrule
\multirow{13}{*}{\rotatebox{90}{ripgrep}} & Literal (mmap, -i) & \scriptsize\textcolor{gray!60}{$\pm$0.000} & 26.069 & \scriptsize\textcolor{gray!60}{$\pm$0.000} & 26.069 \\
 & Literal (default) & \scriptsize\textcolor{gray!60}{$\pm$0.000} & 26.069 & \scriptsize\textcolor{gray!60}{$\pm$0.000} & 26.069 \\
 & Literal (mmap) & \scriptsize\textcolor{gray!60}{$\pm$0.000} & 26.069 & \scriptsize\textcolor{gray!60}{$\pm$0.000} & 26.069 \\
 & Literal (regex) & \scriptsize\textcolor{gray!60}{$\pm$0.000} & 26.069 & \scriptsize\textcolor{gray!60}{$\pm$0.000} & 26.069 \\
 & Literal (-i) & \scriptsize\textcolor{gray!60}{$\pm$0.000} & 26.069 & \scriptsize\textcolor{gray!60}{$\pm$0.000} & 26.069 \\
 & UTF Greek & \scriptsize\textcolor{gray!60}{$\pm$0.000} & 26.069 & \scriptsize\textcolor{gray!60}{$\pm$0.000} & 26.069 \\
 & UTF Greek (-i) & \scriptsize\textcolor{gray!60}{$\pm$0.000} & 26.069 & \scriptsize\textcolor{gray!60}{$\pm$0.000} & 26.069 \\
 & UTF Word & \scriptsize\textcolor{gray!60}{$\pm$0.000} & 26.069 & \scriptsize\textcolor{gray!60}{$\pm$0.000} & 26.069 \\
 & UTF Word (alt.) & \scriptsize\textcolor{gray!60}{$\pm$0.000} & 26.069 & \scriptsize\textcolor{gray!60}{$\pm$0.000} & 26.069 \\
 & Word & \scriptsize\textcolor{gray!60}{$\pm$0.000} & 26.069 & \scriptsize\textcolor{gray!60}{$\pm$0.000} & 26.069 \\
 & Literal & \scriptsize\textcolor{gray!60}{$\pm$0.000} & 26.069 & \scriptsize\textcolor{gray!60}{$\pm$0.000} & 26.069 \\
 & Alternates & \scriptsize\textcolor{gray!60}{$\pm$0.000} & 26.069 & \scriptsize\textcolor{gray!60}{$\pm$0.000} & 26.069 \\
 & Alternates (-i) & \scriptsize\textcolor{gray!60}{$\pm$0.000} & 26.069 & \scriptsize\textcolor{gray!60}{$\pm$0.000} & 26.069 \\
\bottomrule
\end{tabular}
