# Supplementary material for: Garbage Collection for Rust: The Finalizer Frontier
Source: arXiv:2504.01841 source file (2025-09-30)
Supplement: Supplementary file 5 [file appendix_elision_pct_elided_1.tex]

\begin{tabular}{ll@{\hspace{6pt}}r@{\hspace{3pt}}l@{\hspace{6pt}}r@{\hspace{3pt}}l}
\toprule
Suite & Benchmark & \multicolumn{4}{c}{\% Fin. Elided} \\
 &  & \multicolumn{2}{c}{Before} & \multicolumn{2}{c}{After} \\
\midrule
\multirow{13}{*}{\rotatebox{90}{ripgrep}} & Alternates & 0.00 &  & 79.04 &  \\
 & Alternates (-i) & 0.00 &  & 79.04 &  \\
 & Literal & 0.00 &  & 79.04 &  \\
 & Literal (-i) & 0.00 &  & 79.04 &  \\
 & Literal (default) & 0.00 &  & 79.04 &  \\
 & Literal (mmap) & 0.00 &  & 79.04 &  \\
 & Literal (mmap, -i) & 0.00 &  & 79.04 &  \\
 & Literal (regex) & 0.00 &  & 79.04 &  \\
 & UTF Greek & 0.00 &  & 79.04 &  \\
 & UTF Greek (-i) & 0.00 &  & 79.04 &  \\
 & UTF Word & 0.00 &  & 79.04 &  \\
 & UTF Word (alt.) & 0.00 &  & 79.04 &  \\
 & Word & 0.00 &  & 79.04 &  \\
\bottomrule
\end{tabular}
