# Supplementary material for: Garbage Collection for Rust: The Finalizer Frontier
Source: arXiv:2504.01841 source file (2025-09-30)
Supplement: Supplementary file 6 [file appendix_elision_total_collections_1.tex]

\begin{tabular}{ll@{\hspace{6pt}}r@{\hspace{3pt}}l@{\hspace{6pt}}r@{\hspace{3pt}}l}
\toprule
Suite & Benchmark & \multicolumn{4}{c}{\# Collections} \\
 &  & \multicolumn{2}{c}{Before} & \multicolumn{2}{c}{After} \\
\midrule
\multirow{13}{*}{\rotatebox{90}{ripgrep}} & Alternates & 101.80 & \scriptsize\textcolor{gray!60}{$\pm$8.05} & 22.03 & \scriptsize\textcolor{gray!60}{$\pm$0.25} \\
 & Alternates (-i) & 99.80 & \scriptsize\textcolor{gray!60}{$\pm$6.58} & 20.13 & \scriptsize\textcolor{gray!60}{$\pm$0.29} \\
 & Literal & 113.80 & \scriptsize\textcolor{gray!60}{$\pm$7.79} & 23.33 & \scriptsize\textcolor{gray!60}{$\pm$0.33} \\
 & Literal (-i) & 113.90 & \scriptsize\textcolor{gray!60}{$\pm$8.74} & 20.80 & \scriptsize\textcolor{gray!60}{$\pm$0.52} \\
 & Literal (default) & 111.33 & \scriptsize\textcolor{gray!60}{$\pm$8.33} & 23.40 & \scriptsize\textcolor{gray!60}{$\pm$0.47} \\
 & Literal (mmap) & 113.10 & \scriptsize\textcolor{gray!60}{$\pm$6.17} & 22.13 & \scriptsize\textcolor{gray!60}{$\pm$0.22} \\
 & Literal (mmap, -i) & 108.13 & \scriptsize\textcolor{gray!60}{$\pm$8.24} & 21.20 & \scriptsize\textcolor{gray!60}{$\pm$0.28} \\
 & Literal (regex) & 111.60 & \scriptsize\textcolor{gray!60}{$\pm$8.86} & 22.90 & \scriptsize\textcolor{gray!60}{$\pm$0.24} \\
 & UTF Greek & 114.07 & \scriptsize\textcolor{gray!60}{$\pm$8.02} & 20.97 & \scriptsize\textcolor{gray!60}{$\pm$0.16} \\
 & UTF Greek (-i) & 111.90 & \scriptsize\textcolor{gray!60}{$\pm$9.38} & 19.87 & \scriptsize\textcolor{gray!60}{$\pm$0.22} \\
 & UTF Word & 109.53 & \scriptsize\textcolor{gray!60}{$\pm$3.77} & 20.07 & \scriptsize\textcolor{gray!60}{$\pm$0.13} \\
 & UTF Word (alt.) & 114.70 & \scriptsize\textcolor{gray!60}{$\pm$9.48} & 22.43 & \scriptsize\textcolor{gray!60}{$\pm$0.41} \\
 & Word & 97.77 & \scriptsize\textcolor{gray!60}{$\pm$7.94} & 22.03 & \scriptsize\textcolor{gray!60}{$\pm$0.31} \\
\bottomrule
\end{tabular}
